# Supplementary material for: TEASER: Token Enhanced Spatial Modeling for Expressions Reconstruction
Source: arXiv:2502.10982 source file (2025-03-02)
Supplement: Supplementary file 1 [file supp-stirling.pdf]

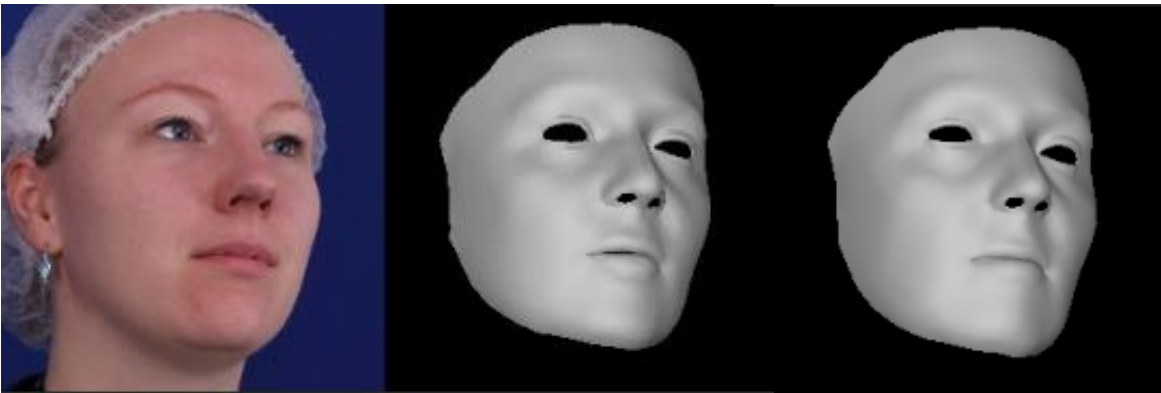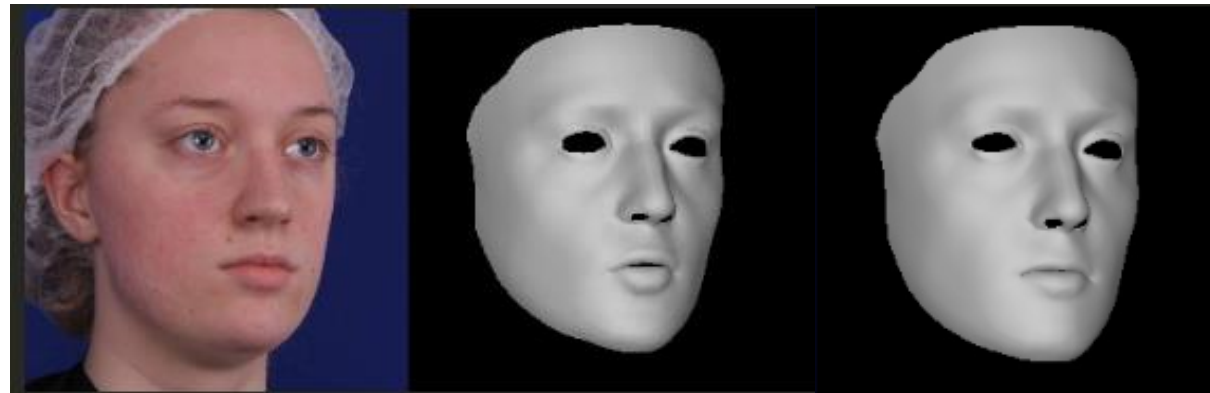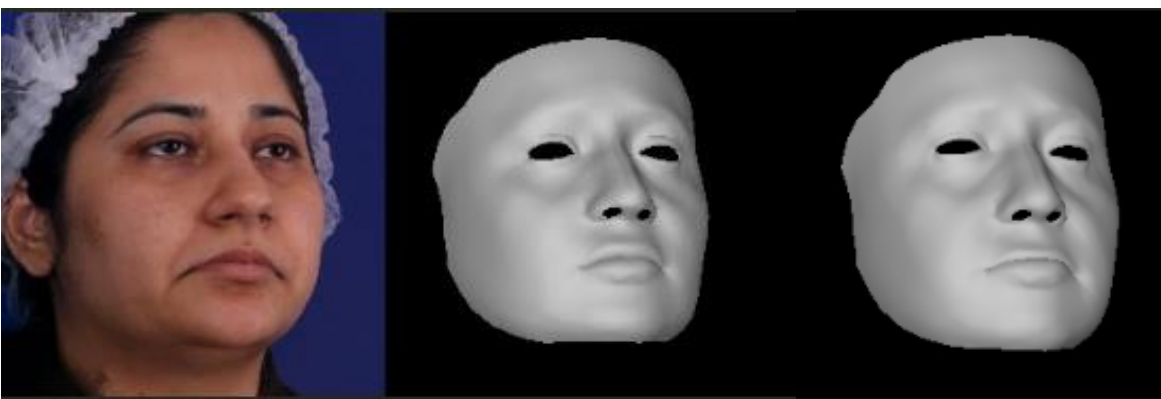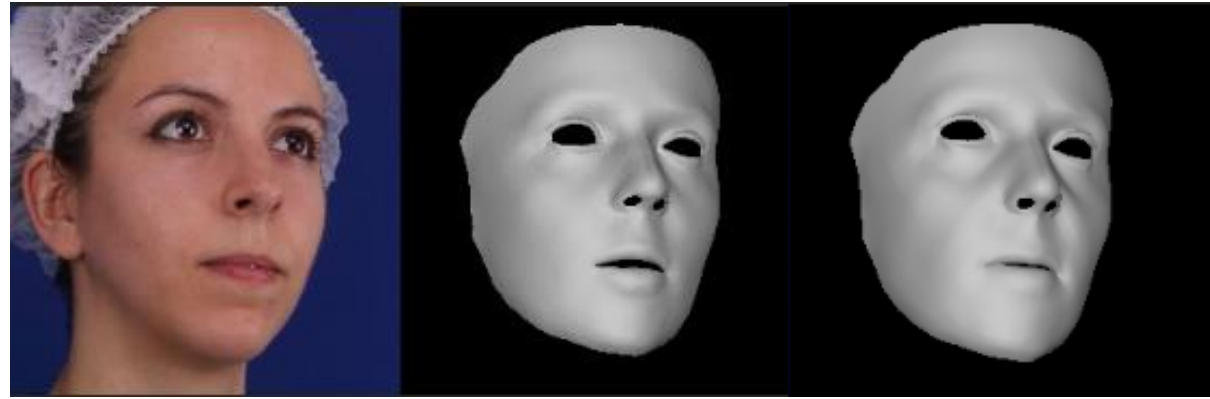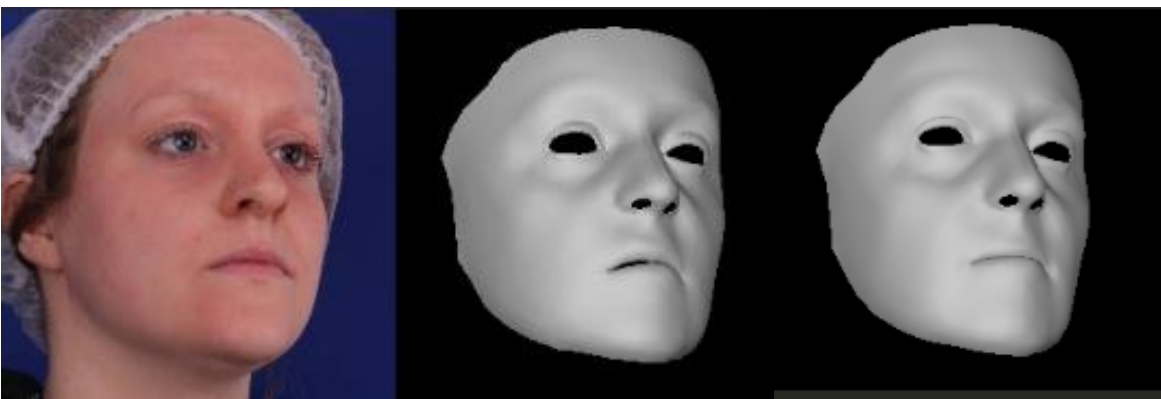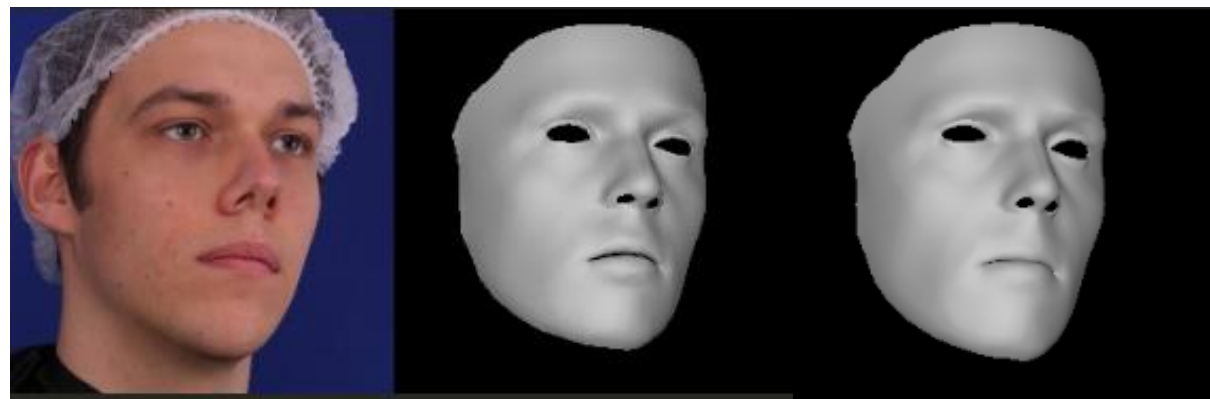

|                 | Median (↓)  | Mean (↓)    | Std (↓)     |
|-----------------|-------------|-------------|-------------|
| Deep3DFaceRecon | 0.99        | 1.27        | 1.15        |
| 3DDFA-v2        | 1.20        | 1.55        | 1.45        |
| DECA            | 1.03        | 1.32        | 1.18        |
| SMIRK           | 1.01        | 1.08        | 1.05        |
| Ours            | <b>1.00</b> | <b>1.07</b> | <b>1.04</b> |
